# Supplementary material for: Computational study of Adhesion and Friction Behavior of Crosslinked Polymer Network
Source: arXiv:2508.21360 ancillary file (2025-08-29)
Supplement: Supplementary file 1 [file Supporting_Information.pdf]

# Supporting Information – "Computational Study of Adhesion and Friction Behavior of Crosslinked Polymer Network"

Ajay Kumar,[1] Manoj Kumar Maurya*,[1] and Manjesh Kumar Singh*,[1]

[1] *Department of Mechanical Engineering, Indian Institute of Technology Kanpur, Kanpur UP 208016, India*

* manojmaurya647@gmail.com
* manjesh@iitk.ac.in

Number of pages: 3
Number of figures: 3
Number of tables: 1

This supplementary document provides additional supporting information for some of the results presented in the main manuscript.

## S1. STRUCTURAL STIFFNESS EVALUATION

To evaluate the structural stiffness, we performed indentation simulations on crosslinked networks with varying fractions of crosslinked monomers ($x_{\rm f}$). The simulations were carried out with an indenter velocity of $0.005\sigma/\tau$, an indenter radius of $r_{\rm ind} = 8.0\sigma$, and an interaction strength of $\epsilon = 1.0$. The stiffness was defined as the initial slope of the unloading curve.

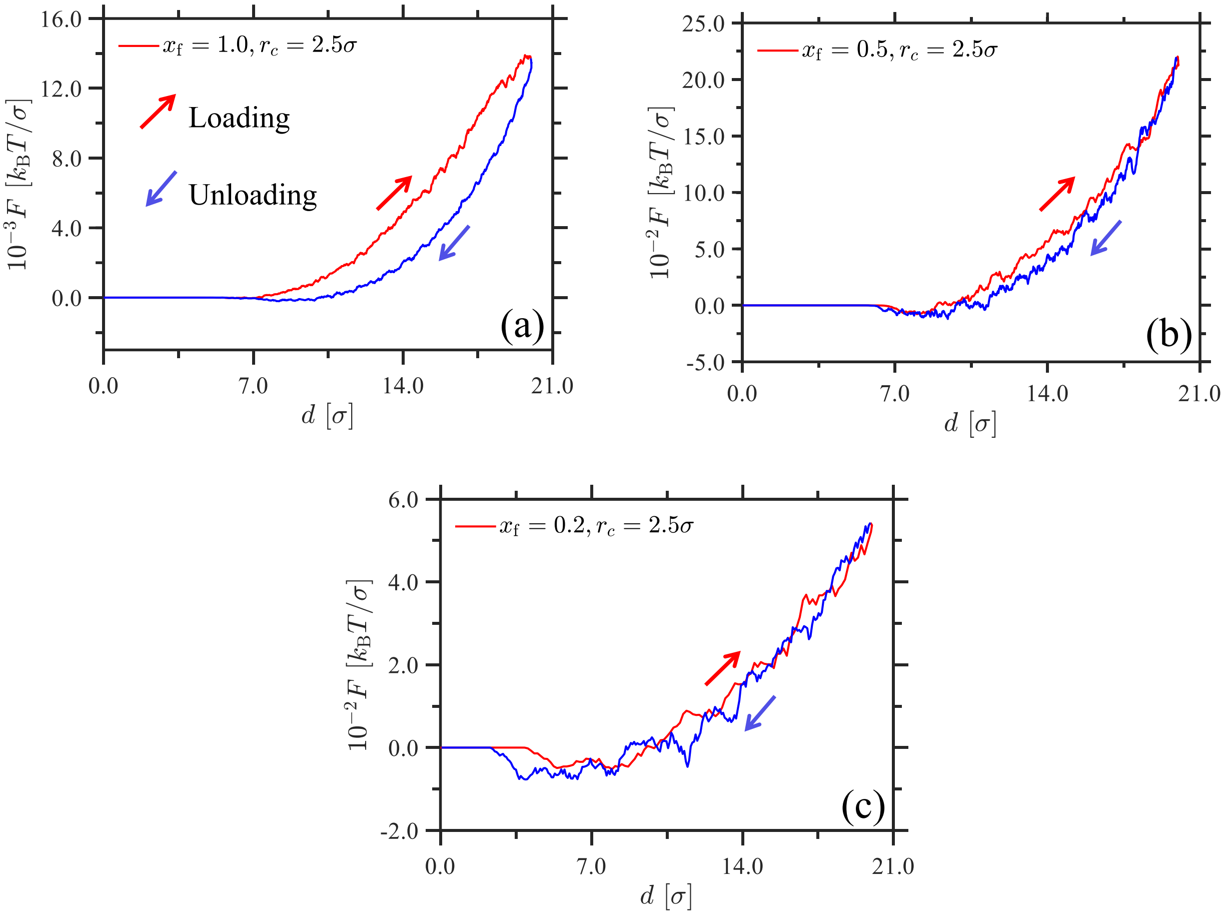


FIG. S1: Loading and unloading plots showing the indentation force $F$ versus indentation depth $d$. The results are presented for a tetrafunctional crosslinked network with different monomer fractions.

## S2. ADHESION ANALYSIS

We performed adhesion analysis for crosslinked networks with varying $x_{\mathrm{f}}$. In this study, we calculated the adhesion (or peeling) force and the separation distance ($S_{\mathrm{d}}$) using an interaction strength of $\epsilon = 2.0$. Figure S2 shows the loading and unloading force as a function of indentation depth. The inset highlights the negative pull-off force that occurs during indenter retraction, measured with a cut-off distance of $r_{\mathrm{c}} = 2.5\sigma$.

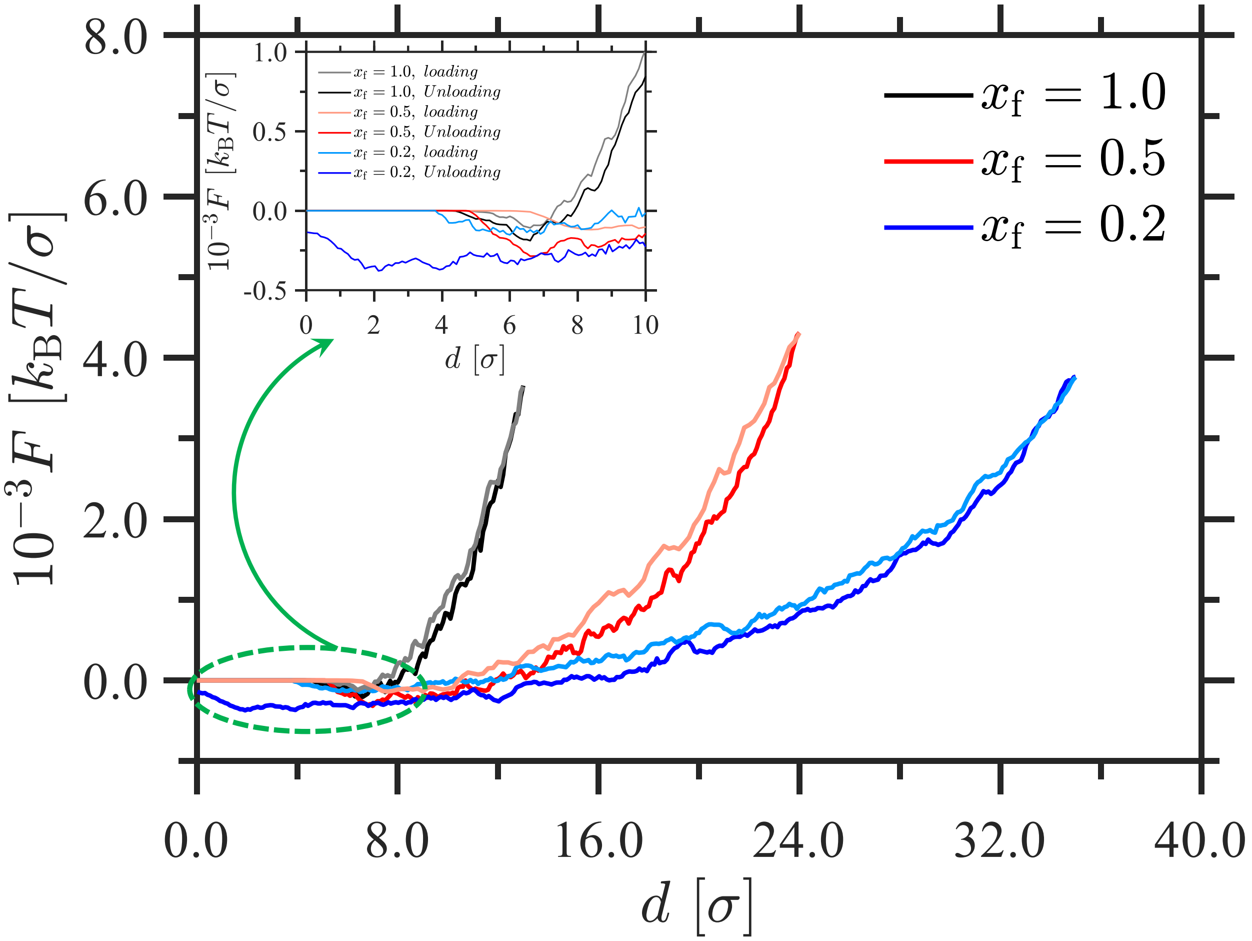


FIG. S2: Loading and unloading force versus indentation depth. The magnified inset in Figure highlights the negative pull-off force observed during indenter unloading of the indenter. Data are shown for tetrafunctional networks with different $x_{\mathrm{f}}$. The indenter approach velocity was $v = 0.005\sigma/\tau$, and the indenter radius was $8.0\sigma$.

## S3. DETERMINATION OF COEFFICIENT OF FRICTION

The coefficient of friction (CoF) and adhesion force ($F_{\mathrm{adh}}$) during sliding were evaluated for crosslinked networks with different values of $x_{\mathrm{f}}$. For each $x_{\mathrm{f}}$, four independent simulations were performed. The system recorded the friction and normal forces, from which average values were computed at various indentation depths. These averaged values were then plotted, and linear regression was applied to the data, as indicated by the dashed lines in corresponding colors in Figure S3.

The regression line is represented by the following equation:

$$F_{\mathrm{f}} = \mu F_{\mathrm{N}} + F_{\mathrm{adh}} \tag{1}$$

Here, $F_{\mathrm{f}}$ is the friction force, $F_{\mathrm{N}}$ is the normal force, $\mu$ is the slope of the fitted line (representing the CoF), and $F_{\mathrm{adh}}$ is the intercept on the y-axis, representing the adhesion force. The extracted data of CoF and adhesion force with different $x_{\mathrm{f}}$ represented in Table S1.

TABLE S1: Friction coefficient and adhesion force for different $x_{\mathrm{f}}$

| $x_{\mathrm{f}}$ | Coefficient of Friction ($\mu$) | Adhesion Force ($F_{\mathrm{adh}}$) [$k_{\mathrm{B}}T/\sigma$] |
|---|---|---|
| 1.0 | 0.2401 | 29.89 |
| 0.5 | 0.2942 | 75.48 |
| 0.2 | 0.4272 | 90.63 |

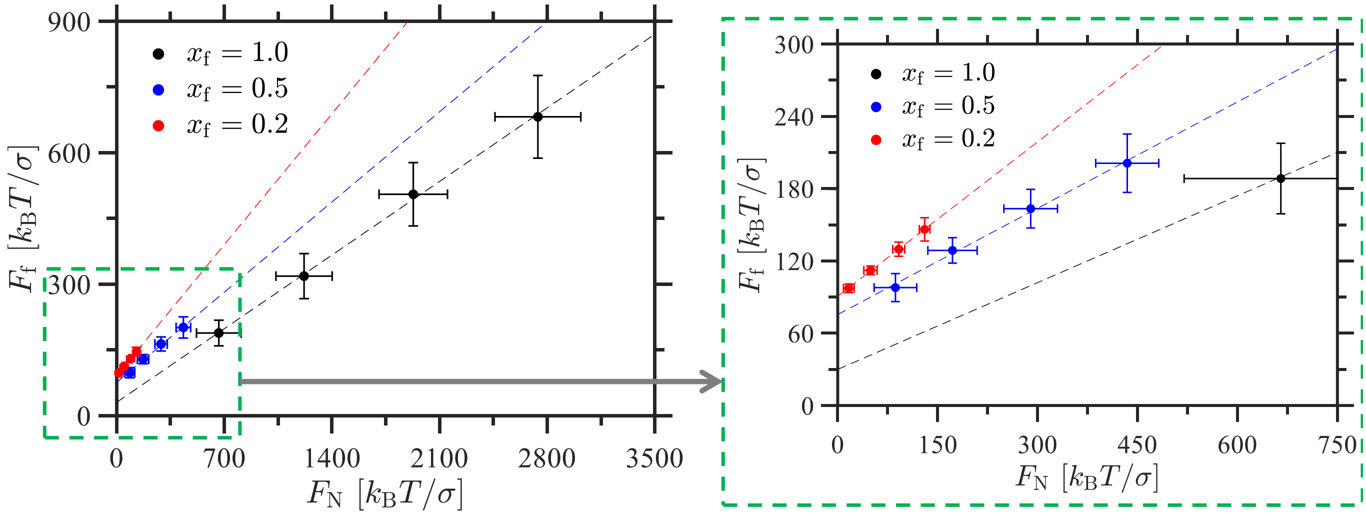


FIG. S3: The average normal force versus friction force data for different values of $x_{\mathrm{f}}$ are shown at various indentation depths during sliding. The dashed lines indicate the linear regression fits for each data set. The inset highlights the average adhesion force corresponding to each $x_{\mathrm{f}}$. All results correspond to tetrafunctional networks, with an indenter approach velocity of $v = 0.005\sigma/\tau$ and an indenter radius of $8.0\sigma$.
